# Supplementary material for: From Hindsight to Foresight: Dissecting Clinical Evidence Acquisition in Large Language Models
Source: arXiv:2610.18605 source file (2026-10-13)
Supplement: Supplementary file 1 [file count-matched.tex]

\begin{tabular}{rrrrrr}
\toprule
Budget & Mean actual facts & Foresight acc. & Matched Hindsight acc. & Gap & 95\% CI \\
\midrule
3 & 2.09 & 33.1\% & 63.0\% & 29.8\% & [22.1\%, 37.6\%] \\
6 & 3.52 & 42.0\% & 70.7\% & 28.7\% & [20.4\%, 37.0\%] \\
\bottomrule
\end{tabular}
