# Supplementary material for: From Hindsight to Foresight: Dissecting Clinical Evidence Acquisition in Large Language Models
Source: arXiv:2610.18605 source file (2026-10-13)
Supplement: Supplementary file 2 [file clinician-agreement.tex]

\begin{tabular}{lrr}
\toprule
Archived slot outcome & Exact agreement & Kappa / ICC \\
\midrule
Top-1 relevance & 100.0\% & n.a. \\
Top-3 critical evidence & 100.0\% & n.a. \\
Top-3 order & 90.0\% & 0.000 \\
Missing-evidence flag & 96.0\% & 0.000 \\
Answer-revealing flag & 96.0\% & 0.000 \\
Preferred Top-1 evidence & 88.0\% & -- \\
Preferred Top-3 evidence & 0.810 Jaccard & -- \\
Quality rating & -- & QWK 0.148; ICC 0.150 \\
Confidence rating & -- & QWK 0.000; ICC 0.000 \\
\bottomrule
\end{tabular}
