# Supplementary material for: From Hindsight to Foresight: Dissecting Clinical Evidence Acquisition in Large Language Models
Source: arXiv:2610.18605 source file (2026-10-13)
Supplement: Supplementary file 3 [file clinician-audit.tex]

\begin{tabular}{lrr}
\toprule
Archived review-record outcome & Estimate & 95\% CI \\
\midrule
Top-1 diagnostically relevant & 100.0\% & [100.0\%, 100.0\%] \\
Top-3 contains critical evidence & 100.0\% & [100.0\%, 100.0\%] \\
Top-3 order reasonable (strict) & 97.5\% & [95.5\%, 99.5\%] \\
Critical evidence missing from Top-3 & 1.0\% & [0.0\%, 2.5\%] \\
Any Top-6 item answer-revealing & 1.0\% & [0.0\%, 2.5\%] \\
Reviewer--Hindsight Top-1 agreement & 89.0\% & [83.0\%, 94.5\%] \\
Reviewer--Hindsight Top-3 Jaccard & 0.870 & [0.829, 0.907] \\
Overall selector quality (1--5) & 4.57 & [4.48, 4.66] \\
\bottomrule
\end{tabular}
